# Supplementary material for: Attention-Based Recurrence for Multi-Agent Reinforcement Learning under Stochastic Partial Observability
Source: arXiv:2301.01649 source file (2023-12-28)
Supplement: Supplementary file 1 [file technical_appendix.tex]

\documentclass{article} % Not really important
\usepackage{pdfpages}
\begin{document}
\includepdf[pages={10-12}]{main.pdf}
\end{document}
